# Supplementary material for: A weight-dependent local correlation density-functional approximation for ensembles
Source: arXiv:2003.05553 source file (2020-05-08)
Supplement: Supplementary file 1 [file eDFT-SI.pdf]

# Supplementary Material for "A weight-dependent local correlation density-functional approximation for ensembles"

Pierre-François Loos[1, a)] and Emmanuel Fromager[2, b)]
[1)]Laboratoire de Chimie et Physique Quantiques (UMR 5626), Université de Toulouse, CNRS, UPS, France
[2)]Laboratoire de Chimie Quantique, Institut de Chimie, CNRS, Université de Strasbourg, Strasbourg, France

## CONSTRUCTION OF THE DENSITY-FUNCTIONAL APPROXIMATIONS

The density-functional approximations designed in this manuscript are based on highly-accurate energies for the ground state ($I = 0$), the first singly-excited state ($I = 1$), and the first doubly-excited state ($I = 2$) of the (spin-polarized) two-electron ringium system (see Fig. 1). We refer the interested reader to Refs. 1–3 for more details about this paradigm.

The reduced (i.e. per electron) HF energy for these three states is:

$$\epsilon_{\text{HF}}^{(0)}(n) = \frac{\pi^2}{8} n^2 + n, \tag{1a}$$

$$\epsilon_{\text{HF}}^{(1)}(n) = \frac{\pi^2}{2} n^2 + \frac{4}{3} n, \tag{1b}$$

$$\epsilon_{\text{HF}}^{(2)}(n) = \frac{9\pi^2}{8} n^2 + \frac{23}{15} n. \tag{1c}$$

All these states have the same (uniform) density $n = 2/(2\pi R)$ where $R$ is the radius of the ring on which the electrons are confined.

The total energy of the ground and doubly-excited states are given by the two lowest eigenvalues of the Hamiltonian $\boldsymbol{H}$

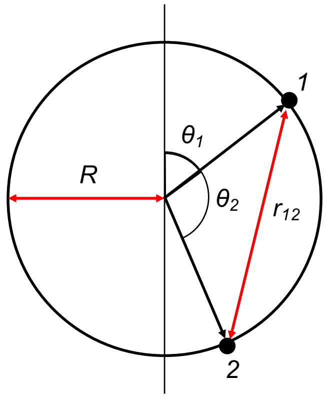


FIG. 1. Schematic representation of two electrons on a ring of radius $R$. $\theta_1$ and $\theta_2$ are the two angles locating the electrons and $r_{12}$ is the interelectronic distance.

a)Electronic mail: loos@irsamc.ups-tlse.fr
b)Electronic mail: fromagere@unistra.fr

with elements

$$\begin{aligned} H_{ij} &= \int_0^\pi \left[ \frac{\psi_i(\omega)}{R} \frac{\psi_j(\omega)}{R} + \frac{\psi_i(\omega)\psi_j(\omega)}{2R\sin(\omega/2)} \right] d\omega \\ &= \frac{\sqrt{\pi}}{2R} \left[ \frac{\Gamma\left(\frac{i+j}{2}\right)}{\Gamma\left(\frac{i+j+1}{2}\right)} + \frac{ij}{4R} \frac{\Gamma\left(\frac{i+j-1}{2}\right)}{\Gamma\left(\frac{i+j+2}{2}\right)} \right], \end{aligned} \tag{2}$$

where $\omega = \theta_1 - \theta_2$ is the interelectronic angle, $\Gamma(x)$ is the Gamma function,[4] and

$$\psi_i(\omega) = \sin(\omega/2) \sin^{i-1}(\omega/2), \quad i = 1, \ldots, M \tag{3}$$

are (non-orthogonal) explicitly-correlated basis functions with overlap matrix elements

$$S_{ij} = \int_0^\pi \psi_i(\omega)\psi_j(\omega) d\omega = \sqrt{\pi} \frac{\Gamma\left(\frac{i+j+1}{2}\right)}{\Gamma\left(\frac{i+j+2}{2}\right)}. \tag{4}$$

Thanks to this explicitly-correlated basis, the convergence rate of the energy is exponential with respect to $M$. Therefore, high accuracy is reached with a very small number of basis functions. Here, we typically use $M = 10$. For the singly-excited state, one has to modify the basis functions as

$$\psi_i(\omega) = \cos(\omega/2) \sin^{i-1}(\omega/2), \tag{5}$$

and its energy is obtained by the lowest root of the Hamiltonian in this basis, and the matrix elements reads

$$H_{ij} = \frac{\sqrt{\pi}}{4R} \left[ \frac{\Gamma\left(\frac{i+j}{2}\right)}{\Gamma\left(\frac{i+j+1}{3}\right)} + \frac{3ij + i + j - 1}{4R} \frac{\Gamma\left(\frac{i+j-1}{2}\right)}{\Gamma\left(\frac{i+j+4}{2}\right)} \right], \tag{6}$$

$$S_{ij} = \frac{\sqrt{\pi}}{2} \frac{\Gamma\left(\frac{i+j+1}{2}\right)}{\Gamma\left(\frac{i+j+4}{2}\right)}. \tag{7}$$

The numerical values of the correlation energy for various $R$ are reported in Table I for the three states of interest.

Based on these highly-accurate calculations, one can write down, for each state, an accurate analytical expression of the reduced correlation energy[2,5] via the following Padé approximant

$$\epsilon_{\text{c}}^{(I)}(n) = \frac{a_1^{(I)}\, n}{n + a_2^{(I)} \sqrt{n} + a_3^{(I)}}, \tag{8}$$

where $a_2^{(I)}$ and $a_3^{(I)}$ are state-specific fitting parameters, which are provided in Table I of the manuscript. The value of $a_1^{(I)}$ is obtained via the exact high-density expansion of the correlation energy.[2,5] Equation (8) is depicted in Fig. 2 for each state

TABLE I. $-\epsilon_c^{(I)}$ as a function of the radius of the ring $R$ for the ground state ($I = 0$), the first singly-excited state ($I = 1$), and the first doubly-excited state ($I = 2$) of the (spin-polarized) two-electron ringium system.

| State | $I$ | Ring's radius $R = 1/(\pi n)$ | | | | | | | | | | |
|---|---|---|---|---|---|---|---|---|---|---|---|---|
| | | 0 | 1/10 | 1/5 | 1/2 | 1 | 2 | 5 | 10 | 20 | 50 | 100 |
| Ground state | 0 | 0.013708 | 0.012859 | 0.012525 | 0.011620 | 0.010374 | 0.008558 | 0.005673 | 0.003697 | 0.002226 | 0.001046 | 0.000567 |
| Singly-excited state | 1 | 0.0238184 | 0.023392 | 0.022979 | 0.021817 | 0.020109 | 0.017371 | 0.012359 | 0.008436 | 0.005257 | 0.002546 | 0.001399 |
| Doubly-excited state | 2 | 0.018715 | 0.018653 | 0.018576 | 0.018300 | 0.017743 | 0.016491 | 0.013145 | 0.009670 | 0.006365 | 0.003231 | 0.001816 |

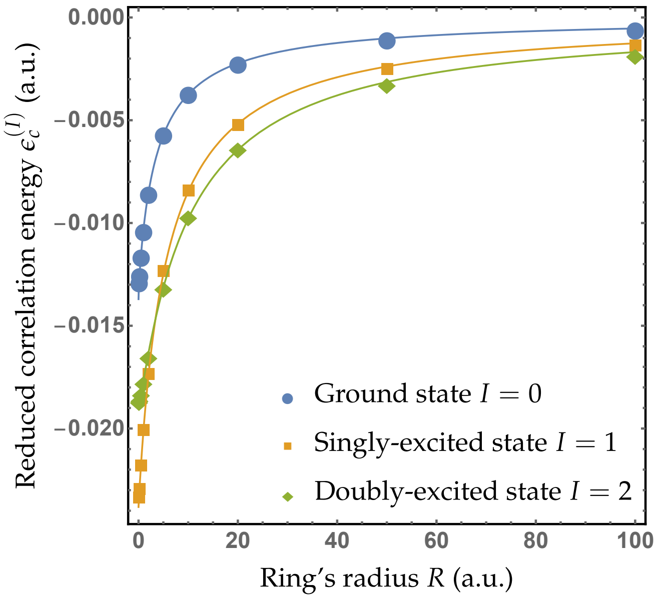


FIG. 2. Reduced (i.e., per electron) correlation energy $\epsilon_c^{(I)}$ [see Eq. (8)] as a function of $R = 1/(\pi n)$ for the ground state ($I = 0$), the first singly-excited state ($I = 1$), and the first doubly-excited state ($I = 2$) of the (spin-polarized) two-electron ringium system. The data gathered in Table I are also reported.

alongside the data gathered in Table I. Note that, in the low-density (*i.e.*, large-$R$ or small-$n$) regime, Eq. (8) has the right behavior, *i.e.*,

$$\epsilon_c^{(I)}(n) = \frac{a_1^{(I)}}{a_3^{(I)}} n - \frac{a_1^{(I)} a_2^{(I)}}{(a_2^{(I)})^2} n^{3/2} + O\left(n^2\right). \tag{9}$$

The two terms in the right-hand-side of Eq. (9) represent the classical repulsion between electrons and their zero-point vibrational energies, respectively. However, their respective coefficients do not match the exact values,[2,5] as these coefficients are determined to reproduce correlation energies at intermediate densities. This has been found to be more practically useful than enforcing the exact low-density values.

[1] P.-F. Loos and P. M. W. Gill, Phys. Rev. Lett. **108**, 083002 (2012).
[2] P.-F. Loos and P. M. W. Gill, J. Chem. Phys. **138**, 164124 (2013).
[3] P.-F. Loos, C. J. Ball, and P. M. W. Gill, J. Chem. Phys. **140**, 18A524 (2014).
[4] F. W. J. Olver, D. W. Lozier, R. F. Boisvert, and C. W. Clark, eds., *NIST Handbook of Mathematical Functions* (Cambridge University Press, New York, 2010).
[5] P.-F. Loos, Phys. Rev. A **89**, 052523 (2014).

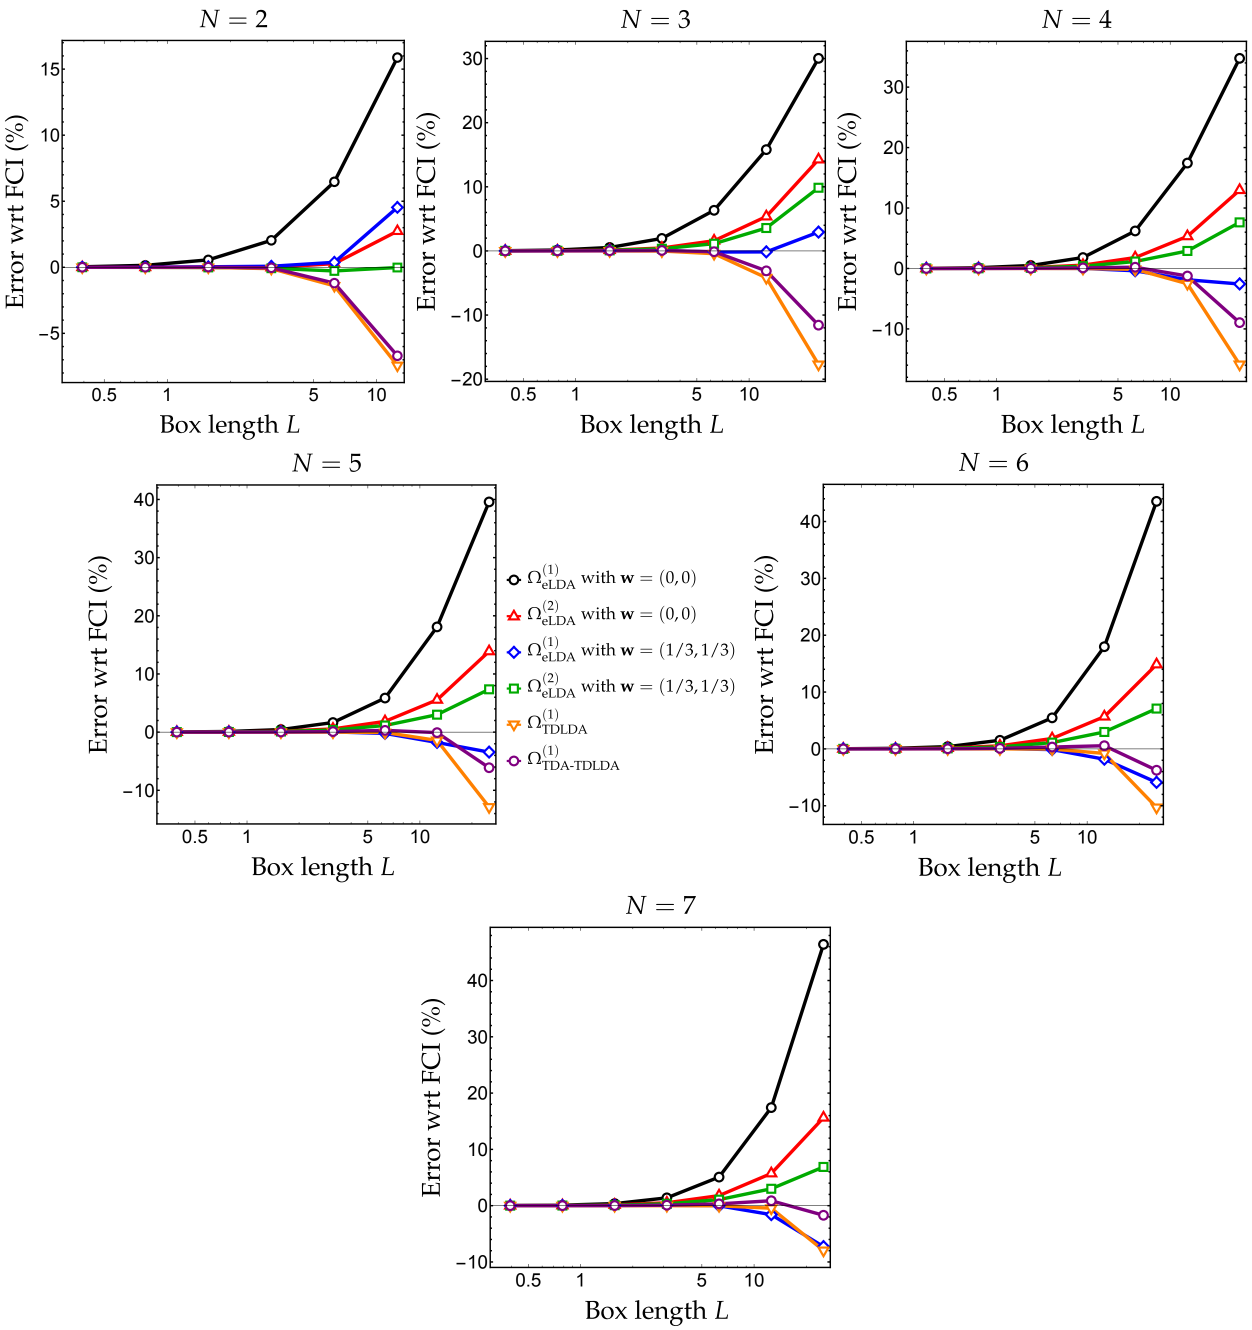


FIG. 3. Error with respect to FCI in single and double excitation energies of $N$-boxium as a function of the box length $L$ for various methods. See main text for additional details.

TABLE II. Deviation from the FCI quantities (in hartree) of the individual energies, $E^{(I)}$, and the corresponding excitation energies, $\Omega^{(I)}$, for the ground ($I = 0$), singly-excited ($I = 1$) and doubly-excited ($I = 2$) states of 2-boxium (i.e., $N = 2$ electrons in a box of length $L$). The values of the ensemble correlation derivative $\Upsilon_c^{(I)}$ are also reported.

| | | | 2-boxium with a box of length $L$ | | | | | | |
|---|---|---|---|---|---|---|---|---|---|
| Method | $\boldsymbol{w}$ | State | $\pi/8$ | $\pi/4$ | $\pi/2$ | $\pi$ | $2\pi$ | $4\pi$ | $8\pi$ |
| FCI | | $E^{(0)}$ | 168.1946 | 44.0662 | 12.0035 | 3.4747 | 1.0896 | 0.3719 | 0.1367 |
| | | $E^{(1)}$ | 330.2471 | 85.0890 | 22.5112 | 6.2247 | 1.8355 | 0.5845 | 0.2006 |
| | | $E^{(2)}$ | 809.9972 | 204.9840 | 52.4777 | 13.7252 | 3.7248 | 1.0696 | 0.3300 |
| | | $\Omega^{(1)}$ | 162.0525 | 41.0228 | 10.5078 | 2.7500 | 0.7458 | 0.2125 | 0.0639 |
| | | $\Omega^{(2)}$ | 641.8026 | 160.9177 | 40.4743 | 10.2505 | 2.6352 | 0.6977 | 0.1933 |
| | | | Deviation from FCI | | | | | | |
| CIS | | $\Omega^{(1)}$ | 0.0104 | 0.0102 | 0.0099 | 0.0092 | 0.0077 | 0.0051 | 0.0022 |
| TDHF | | $\Omega^{(1)}$ | 0.0019 | 0.0021 | 0.0023 | 0.0027 | 0.0029 | 0.0023 | 0.0011 |
| TDA-TDLDA | | $\Omega^{(1)}$ | 0.0099 | 0.0088 | 0.0058 | −0.0041 | −0.0316 | −0.0467 | |
| TDLDA | | $\Omega^{(1)}$ | 0.0015 | 0.0006 | −0.0018 | −0.0106 | −0.0370 | −0.0518 | |
| KS-eLDA | $(0, 0)$ | $E^{(0)}$ | −0.0397 | −0.0391 | −0.0380 | −0.0361 | −0.0323 | −0.0236 | |
| | | $E^{(1)}$ | 0.0215 | 0.0213 | 0.0210 | 0.0200 | 0.0159 | 0.0102 | |
| | | $E^{(2)}$ | −0.0426 | −0.0425 | −0.0419 | −0.0387 | −0.0250 | −0.0045 | |
| | | $\Omega^{(1)}$ | 0.0612 | 0.0604 | 0.0590 | 0.0561 | 0.0483 | 0.0337 | |
| | | $\Omega^{(2)}$ | −0.0029 | −0.0034 | −0.0039 | −0.0025 | 0.0074 | 0.0191 | |
| | | $\Upsilon_c^{(0)}$ | 0.0000 | 0.0000 | 0.0000 | 0.0000 | 0.0000 | 0.0000 | |
| | | $\Upsilon_c^{(1)}$ | 0.0064 | 0.0056 | 0.0043 | 0.0022 | −0.0007 | −0.0037 | |
| | | $\Upsilon_c^{(2)}$ | 0.0159 | 0.0147 | 0.0126 | 0.0093 | 0.0046 | −0.0009 | |
| KS-eLDA | $(1/3, 1/3)$ | $E^{(0)}$ | 0.0031 | 0.0036 | 0.0044 | 0.0054 | 0.0042 | −0.0025 | |
| | | $E^{(1)}$ | 0.0090 | 0.0087 | 0.0083 | 0.0076 | 0.0070 | 0.0071 | |
| | | $E^{(2)}$ | −0.0005 | −0.0009 | −0.0015 | −0.0023 | −0.0030 | −0.0026 | |
| | | $\Omega^{(1)}$ | 0.0058 | 0.0052 | 0.0039 | 0.0022 | 0.0028 | 0.0096 | |
| | | $\Omega^{(2)}$ | −0.0036 | −0.0045 | −0.0058 | −0.0077 | −0.0072 | 0.0000 | |
| | | $\Upsilon_c^{(0)}$ | −0.0074 | −0.0067 | −0.0055 | −0.0036 | −0.0010 | 0.0019 | |
| | | $\Upsilon_c^{(1)}$ | −0.0010 | −0.0011 | −0.0014 | −0.0017 | −0.0021 | −0.0022 | |
| | | $\Upsilon_c^{(2)}$ | 0.0084 | 0.0079 | 0.0069 | 0.0053 | 0.0031 | 0.0003 | |

TABLE III. Deviation from the FCI quantities (in hartree) of the individual energies, $E^{(I)}$, and the corresponding excitation energies, $\Omega^{(I)}$, for the ground ($I = 0$), singly-excited ($I = 1$) and doubly-excited ($I = 2$) states of 3-boxium (i.e., $N = 3$ electrons in a box of length $L$). The values of the ensemble correlation derivative $\Upsilon_c^{(I)}$ are also reported.

| | | | 3-boxium with a box of length $L$ | | | | | | |
|---|---|---|---|---|---|---|---|---|---|
| Method | $\boldsymbol{w}$ | State | $\pi/8$ | $\pi/4$ | $\pi/2$ | $\pi$ | $2\pi$ | $4\pi$ | $8\pi$ |
| FCI | | $E^{(0)}$ | 475.6891 | 125.7776 | 34.8248 | 10.3536 | 3.3766 | 1.2126 | 0.4721 |
| | | $E^{(1)}$ | 702.8330 | 183.3370 | 49.5922 | 14.2255 | 4.4269 | 1.5105 | 0.5606 |
| | | $E^{(2)}$ | 1379.3128 | 353.5967 | 92.7398 | 25.3135 | 7.3546 | 2.3203 | 0.7990 |
| | | $\Omega^{(1)}$ | 227.1438 | 57.5594 | 14.7674 | 3.8720 | 1.0504 | 0.2979 | 0.0885 |
| | | $\Omega^{(2)}$ | 903.6236 | 227.8191 | 57.9150 | 14.9599 | 3.9780 | 1.1077 | 0.3269 |
| | | | Deviation from FCI | | | | | | |
| TDA-TDLDA | | $\Omega^{(1)}$ | 0.0162 | 0.0157 | 0.0146 | 0.0110 | −0.0049 | −0.0344 | −0.0378 |
| TDLDA | | $\Omega^{(1)}$ | 0.0262 | 0.0264 | 0.0264 | 0.0269 | 0.0273 | 0.0206 | −0.0116 |
| KS-eLDA | $(0, 0)$ | $E^{(0)}$ | −0.0481 | −0.0478 | −0.0473 | −0.0463 | −0.0446 | −0.0387 | −0.0257 |
| | | $E^{(1)}$ | 0.0343 | 0.0336 | 0.0321 | 0.0292 | 0.0220 | 0.0084 | 0.0008 |
| | | $E^{(2)}$ | 0.0277 | 0.0267 | 0.0247 | 0.0216 | 0.0187 | 0.0208 | 0.0209 |
| | | $\Omega^{(1)}$ | 0.0824 | 0.0814 | 0.0794 | 0.0755 | 0.0666 | 0.0471 | 0.0266 |
| | | $\Omega^{(2)}$ | 0.0759 | 0.0745 | 0.0720 | 0.0679 | 0.0633 | 0.0595 | 0.0467 |
| | | $\Upsilon_c^{(0)}$ | 0.0000 | 0.0000 | 0.0000 | 0.0000 | 0.0000 | 0.0000 | 0.0000 |
| | | $\Upsilon_c^{(1)}$ | 0.0100 | 0.0092 | 0.0077 | 0.0051 | 0.0012 | −0.0034 | −0.0072 |
| | | $\Upsilon_c^{(2)}$ | 0.0244 | 0.0231 | 0.0208 | 0.0168 | 0.0108 | 0.0029 | −0.0050 |
| KS-eLDA | $(1/3, 1/3)$ | $E^{(0)}$ | 0.0078 | 0.0080 | 0.0082 | 0.0085 | 0.0081 | 0.0024 | −0.0022 |
| | | $E^{(1)}$ | 0.0172 | 0.0162 | 0.0144 | 0.0112 | 0.0064 | 0.0019 | 0.0004 |
| | | $E^{(2)}$ | 0.0645 | 0.0636 | 0.0621 | 0.0590 | 0.0530 | 0.0420 | 0.0300 |
| | | $\Omega^{(1)}$ | 0.0094 | 0.0083 | 0.0062 | 0.0027 | −0.0018 | −0.0004 | 0.0026 |
| | | $\Omega^{(2)}$ | 0.0567 | 0.0557 | 0.0539 | 0.0506 | 0.0449 | 0.0397 | 0.0323 |
| | | $\Upsilon_c^{(0)}$ | −0.0115 | −0.0107 | −0.0094 | −0.0072 | −0.0038 | 0.0005 | 0.0045 |
| | | $\Upsilon_c^{(1)}$ | −0.0015 | −0.0016 | −0.0018 | −0.0022 | −0.0028 | −0.0033 | −0.0032 |
| | | $\Upsilon_c^{(2)}$ | 0.0129 | 0.0123 | 0.0113 | 0.0094 | 0.0066 | 0.0028 | −0.0013 |

TABLE IV. Deviation from the FCI quantities (in hartree) of the individual energies, $E^{(I)}$, and the corresponding excitation energies, $\Omega^{(I)}$, for the ground ($I = 0$), singly-excited ($I = 1$) and doubly-excited ($I = 2$) states of 4-boxium (i.e., $N = 4$ electrons in a box of length $L$). The values of the ensemble correlation derivative $\Upsilon_c^{(I)}$ are also reported.

| | | | 4-boxium with a box of length $L$ | | | | | | |
|---|---|---|---|---|---|---|---|---|---|
| Method | $\boldsymbol{w}$ | State | $\pi/8$ | $\pi/4$ | $\pi/2$ | $\pi$ | $2\pi$ | $4\pi$ | $8\pi$ |
| FCI | | $E^{(0)}$ | 1020.3778 | 270.0849 | 74.9426 | 22.3790 | 7.3595 | 2.6798 | 1.0633 |
| | | $E^{(1)}$ | 1312.2776 | 344.0184 | 93.8936 | 27.3398 | 8.7021 | 3.0600 | 1.1764 |
| | | $E^{(2)}$ | 2183.4399 | 563.5949 | 149.6753 | 41.7213 | 12.5052 | 4.1033 | 1.4749 |
| | | $\Omega^{(1)}$ | 291.8998 | 73.9335 | 18.9510 | 4.9608 | 1.3426 | 0.3802 | 0.1131 |
| | | $\Omega^{(2)}$ | 1163.0621 | 293.5099 | 74.7326 | 19.3423 | 5.1457 | 1.4235 | 0.4116 |
| | | | Deviation from FCI | | | | | | |
| TDA-TDLDA | | $\Omega^{(1)}$ | 0.0203 | 0.0201 | 0.0195 | 0.0181 | 0.0106 | −0.0178 | −0.0369 |
| TDLDA | | $\Omega^{(1)}$ | 0.0008 | 0.0007 | 0.0004 | −0.0006 | −0.0074 | −0.0360 | −0.0653 |
| KS-eLDA | $(0,0)$ | $E^{(0)}$ | −0.0541 | −0.0539 | −0.0537 | −0.0534 | −0.0529 | −0.0504 | −0.0386 |
| | | $E^{(1)}$ | 0.0413 | 0.0406 | 0.0390 | 0.0362 | 0.0304 | 0.0159 | 0.0008 |
| | | $E^{(2)}$ | 0.0642 | 0.0622 | 0.0586 | 0.0517 | 0.0399 | 0.0254 | 0.0149 |
| | | $\Omega^{(1)}$ | 0.0954 | 0.0945 | 0.0927 | 0.0896 | 0.0833 | 0.0663 | 0.0394 |
| | | $\Omega^{(2)}$ | 0.1182 | 0.1162 | 0.1123 | 0.1051 | 0.0928 | 0.0758 | 0.0534 |
| | | $\Upsilon_c^{(0)}$ | 0.0000 | 0.0000 | 0.0000 | 0.0000 | 0.0000 | 0.0000 | 0.0000 |
| | | $\Upsilon_c^{(1)}$ | 0.0136 | 0.0127 | 0.0111 | 0.0083 | 0.0038 | −0.0022 | −0.0080 |
| | | $\Upsilon_c^{(2)}$ | 0.0330 | 0.0316 | 0.0291 | 0.0248 | 0.0178 | 0.0080 | −0.0028 |
| KS-eLDA | $(1/3,1/3)$ | $E^{(0)}$ | 0.0085 | 0.0085 | 0.0084 | 0.0082 | 0.0072 | 0.0021 | −0.0015 |
| | | $E^{(1)}$ | 0.0164 | 0.0152 | 0.0129 | 0.0087 | 0.0020 | −0.0050 | −0.0044 |
| | | $E^{(2)}$ | 0.0936 | 0.0917 | 0.0880 | 0.0807 | 0.0664 | 0.0434 | 0.0300 |
| | | $\Omega^{(1)}$ | 0.0079 | 0.0067 | 0.0045 | 0.0006 | −0.0051 | −0.0071 | −0.0029 |
| | | $\Omega^{(2)}$ | 0.0851 | 0.0832 | 0.0796 | 0.0725 | 0.0593 | 0.0413 | 0.0315 |
| | | $\Upsilon_c^{(0)}$ | −0.0155 | −0.0148 | −0.0134 | −0.0110 | −0.0071 | −0.0017 | 0.0040 |
| | | $\Upsilon_c^{(1)}$ | −0.0020 | −0.0021 | −0.0023 | −0.0027 | −0.0034 | −0.0042 | −0.0044 |
| | | $\Upsilon_c^{(2)}$ | 0.0175 | 0.0168 | 0.0157 | 0.0137 | 0.0105 | 0.0059 | 0.0004 |

TABLE V. Deviation from the FCI quantities (in hartree) of the individual energies, $E^{(I)}$, and the corresponding excitation energies, $\Omega^{(I)}$, for the ground ($I = 0$), singly-excited ($I = 1$) and doubly-excited ($I = 2$) states of 5-boxium (i.e., $N = 5$ electrons in a box of length $L$). The values of the ensemble correlation derivative $\Upsilon_c^{(I)}$ are also reported.

| | | | 5-boxium with a box of length $L$ | | | | | | |
|---|---|---|---|---|---|---|---|---|---|
| Method | $\boldsymbol{w}$ | State | $\pi/8$ | $\pi/4$ | $\pi/2$ | $\pi$ | $2\pi$ | $4\pi$ | $8\pi$ |
| FCI | | $E^{(0)}$ | 1867.6344 | 493.6760 | 136.7020 | 40.7244 | 13.3763 | 4.8811 | 1.9492 |
| | | $E^{(1)}$ | 2224.11488 | 583.8981 | 159.7957 | 46.7553 | 15.0029 | 5.3399 | 2.0855 |
| | | $E^{(2)}$ | 3289.2022 | 852.4249 | 228.0415 | 64.3597 | 19.6613 | 6.6206 | 2.4547 |
| | | $\Omega^{(1)}$ | 356.4804 | 90.2221 | 23.0937 | 6.0308 | 1.6266 | 0.4588 | 0.1363 |
| | | $\Omega^{(2)}$ | 1421.56773 | 358.7489 | 91.3395 | 23.6352 | 6.2850 | 1.7395 | 0.5055 |
| | | | Deviation from FCI | | | | | | |
| TDA-TDLDA | | $\Omega^{(1)}$ | 0.0230 | 0.0230 | 0.0228 | 0.0223 | 0.0192 | −0.0015 | −0.0309 |
| TDLDA | | $\Omega^{(1)}$ | 0.0005 | 0.0005 | 0.0004 | 0.0000 | −0.0033 | −0.0248 | −0.0650 |
| KS-eLDA | $(0, 0)$ | $E^{(0)}$ | −0.0587 | −0.0586 | −0.0587 | −0.0588 | −0.0591 | −0.0590 | −0.0506 |
| | | $E^{(1)}$ | 0.0457 | 0.0450 | 0.0435 | 0.0409 | 0.0362 | 0.0241 | 0.0033 |
| | | $E^{(2)}$ | 0.0861 | 0.0838 | 0.0793 | 0.0712 | 0.0571 | 0.0377 | 0.0196 |
| | | $\Omega^{(1)}$ | 0.1044 | 0.1036 | 0.1022 | 0.0997 | 0.0953 | 0.0830 | 0.0540 |
| | | $\Omega^{(2)}$ | 0.1447 | 0.1424 | 0.1380 | 0.1300 | 0.1162 | 0.0966 | 0.0703 |
| | | $\Upsilon_c^{(0)}$ | 0.0000 | 0.0000 | 0.0000 | 0.0000 | 0.0000 | 0.0000 | 0.0000 |
| | | $\Upsilon_c^{(1)}$ | 0.0172 | 0.0163 | 0.0147 | 0.0117 | 0.0067 | −0.0004 | −0.0080 |
| | | $\Upsilon_c^{(2)}$ | 0.0416 | 0.0402 | 0.0376 | 0.0329 | 0.0253 | 0.0140 | 0.0005 |
| KS-eLDA | $(1/3, 1/3)$ | $E^{(0)}$ | 0.0070 | 0.0070 | 0.0068 | 0.0063 | 0.0053 | 0.0015 | −0.0049 |
| | | $E^{(1)}$ | 0.0162 | 0.0151 | 0.0128 | 0.0086 | 0.0018 | −0.0066 | −0.0095 |
| | | $E^{(2)}$ | 0.1080 | 0.1056 | 0.1011 | 0.0925 | 0.0772 | 0.0538 | 0.0325 |
| | | $\Omega^{(1)}$ | 0.0092 | 0.0081 | 0.0060 | 0.0022 | −0.0035 | −0.0081 | −0.0047 |
| | | $\Omega^{(2)}$ | 0.1010 | 0.0986 | 0.0943 | 0.0862 | 0.0719 | 0.0523 | 0.0373 |
| | | $\Upsilon_c^{(0)}$ | −0.0196 | −0.0188 | −0.0174 | −0.0148 | −0.0106 | −0.0044 | 0.0029 |
| | | $\Upsilon_c^{(1)}$ | −0.0024 | −0.0025 | −0.0027 | −0.0032 | −0.0040 | −0.0050 | −0.0056 |
| | | $\Upsilon_c^{(2)}$ | 0.0220 | 0.0213 | 0.0201 | 0.0180 | 0.0146 | 0.0093 | 0.0027 |

TABLE VI. Deviation from the FCI quantities (in hartree) of the individual energies, $E^{(I)}$, and the corresponding excitation energies, $\Omega^{(I)}$, for the ground ($I = 0$), singly-excited ($I = 1$) and doubly-excited ($I = 2$) states of 6-boxium (i.e., $N = 6$ electrons in a box of length $L$). The values of the ensemble correlation derivative $\Upsilon_c^{(I)}$ are also reported.

| | | | 6-boxium with a box of length $L$ | | | | | | |
|---|---|---|---|---|---|---|---|---|---|
| Method | $\boldsymbol{w}$ | State | $\pi/8$ | $\pi/4$ | $\pi/2$ | $\pi$ | $2\pi$ | $4\pi$ | $8\pi$ |
| FCI | | $E^{(0)}$ | 3082.5386 | 813.0910 | 224.3734 | 66.5257 | 21.7454 | 7.9136 | 3.1633 |
| | | $E^{(1)}$ | 3503.4911 | 919.5487 | 251.5842 | 73.6145 | 23.6504 | 8.4487 | 3.3217 |
| | | $E^{(2)}$ | 4762.0921 | 1236.8257 | 332.1993 | 94.3988 | 29.1455 | 9.9582 | 3.7572 |
| | | $\Omega^{(1)}$ | 420.9525 | 106.4577 | 27.2108 | 7.0888 | 1.9050 | 0.5351 | 0.1583 |
| | | $\Omega^{(2)}$ | 1679.5536 | 423.7347 | 107.8259 | 27.8731 | 7.4001 | 2.0446 | 0.5938 |
| | | | Deviation from FCI | | | | | | |
| TDA-TDLDA | | $\Omega^{(1)}$ | 0.0249 | 0.0248 | 0.0250 | 0.0250 | 0.0242 | 0.0114 | −0.0223 |
| TDLDA | | $\Omega^{(1)}$ | 0.0002 | 0.0000 | 0.0002 | 0.0000 | −0.0016 | −0.0162 | −0.0612 |
| KS-eLDA | $(0, 0)$ | $E^{(0)}$ | −0.0626 | −0.0627 | −0.0628 | −0.0632 | −0.0641 | −0.0654 | −0.0612 |
| | | $E^{(1)}$ | 0.0486 | 0.0477 | 0.0465 | 0.0440 | 0.0400 | 0.0308 | 0.0078 |
| | | $E^{(2)}$ | 0.1017 | 0.0992 | 0.0946 | 0.0862 | 0.0718 | 0.0507 | 0.0271 |
| | | $\Omega^{(1)}$ | 0.1112 | 0.1104 | 0.1093 | 0.1072 | 0.1041 | 0.0962 | 0.0690 |
| | | $\Omega^{(2)}$ | 0.1643 | 0.1619 | 0.1575 | 0.1494 | 0.1358 | 0.1162 | 0.0884 |
| | | $\Upsilon_c^{(0)}$ | 0.0000 | 0.0000 | 0.0000 | 0.0000 | 0.0000 | 0.0000 | 0.0000 |
| | | $\Upsilon_c^{(1)}$ | 0.0208 | 0.0199 | 0.0182 | 0.0151 | 0.0098 | 0.0018 | −0.0075 |
| | | $\Upsilon_c^{(2)}$ | 0.0503 | 0.0488 | 0.0460 | 0.0412 | 0.0330 | 0.0205 | 0.0046 |
| KS-eLDA | $(1/3, 1/3)$ | $E^{(0)}$ | 0.0046 | 0.0045 | 0.0043 | 0.0039 | 0.0031 | 0.0006 | −0.0067 |
| | | $E^{(1)}$ | 0.0157 | 0.0144 | 0.0123 | 0.0080 | 0.0009 | −0.0091 | −0.0160 |
| | | $E^{(2)}$ | 0.1167 | 0.1142 | 0.1095 | 0.1007 | 0.0853 | 0.0616 | 0.0355 |
| | | $\Omega^{(1)}$ | 0.0112 | 0.0099 | 0.0080 | 0.0041 | −0.0022 | −0.0097 | −0.0093 |
| | | $\Omega^{(2)}$ | 0.1121 | 0.1097 | 0.1051 | 0.0968 | 0.0822 | 0.0610 | 0.0423 |
| | | $\Upsilon_c^{(0)}$ | −0.0237 | −0.0229 | −0.0214 | −0.0188 | −0.0142 | −0.0073 | 0.0013 |
| | | $\Upsilon_c^{(1)}$ | −0.0029 | −0.0030 | −0.0032 | −0.0037 | −0.0045 | −0.0057 | −0.0066 |
| | | $\Upsilon_c^{(2)}$ | 0.0266 | 0.0259 | 0.0246 | 0.0224 | 0.0187 | 0.0130 | 0.0053 |

TABLE VII. Deviation from the FCI quantities (in hartree) of the individual energies, $E^{(I)}$, and the corresponding excitation energies, $\Omega^{(I)}$, for the ground ($I = 0$), singly-excited ($I = 1$) and doubly-excited ($I = 2$) states of 7-boxium (i.e., $N = 7$ electrons in a box of length $L$). The values of the ensemble correlation derivative $\Upsilon_c^{(I)}$ are also reported.

| | | | 7-boxium with a box of length $L$ | | | | | | |
|---|---|---|---|---|---|---|---|---|---|
| Method | $\boldsymbol{w}$ | State | $\pi/8$ | $\pi/4$ | $\pi/2$ | $\pi$ | $2\pi$ | $4\pi$ | $8\pi$ |
| FCI | | $E^{(0)}$ | 4729.98018 | 1244.7753 | 342.1796 | 100.8943 | 32.7728 | 11.8683 | 4.7359 |
| | | $E^{(1)}$ | 5215.3307 | 1367.4316 | 373.4897 | 109.0326 | 34.9524 | 12.4779 | 4.9156 |
| | | $E^{(2)}$ | 6667.18516 | 1733.3319 | 466.4133 | 132.9686 | 41.2715 | 14.2096 | 5.4146 |
| | | $\Omega^{(1)}$ | 485.3505 | 122.6563 | 31.3101 | 8.1382 | 2.1796 | 0.6096 | 0.1797 |
| | | $\Omega^{(2)}$ | 1937.2050 | 488.5566 | 124.2336 | 32.0743 | 8.4987 | 2.3413 | 0.6787 |
| | | | Deviation from FCI | | | | | | |
| TDA-TDLDA | | $\Omega^{(1)}$ | 0.0262 | 0.0264 | 0.0264 | 0.0269 | 0.0273 | 0.0206 | −0.0116 |
| TDLDA | | $\Omega^{(1)}$ | 0.0000 | 0.0001 | 0.0000 | −0.0001 | −0.0009 | −0.0107 | −0.0539 |
| KS-eLDA | $(0, 0)$ | $E^{(0)}$ | −0.0664 | −0.0666 | −0.0667 | −0.0672 | −0.0684 | −0.0707 | −0.0702 |
| | | $E^{(1)}$ | 0.0502 | 0.0495 | 0.0482 | 0.0459 | 0.0423 | 0.0355 | 0.0131 |
| | | $E^{(2)}$ | 0.1122 | 0.1104 | 0.1061 | 0.0979 | 0.0836 | 0.0635 | 0.0360 |
| | | $\Omega^{(1)}$ | 0.1165 | 0.1161 | 0.1149 | 0.1131 | 0.1108 | 0.1062 | 0.0834 |
| | | $\Omega^{(2)}$ | 0.1785 | 0.1769 | 0.1728 | 0.1652 | 0.1520 | 0.1342 | 0.1063 |
| | | $\Upsilon_c^{(0)}$ | 0.0000 | 0.0000 | 0.0000 | 0.0000 | 0.0000 | 0.0000 | 0.0000 |
| | | $\Upsilon_c^{(1)}$ | 0.0244 | 0.0235 | 0.0218 | 0.0186 | 0.0130 | 0.0043 | −0.0065 |
| | | $\Upsilon_c^{(2)}$ | 0.0589 | 0.0574 | 0.0546 | 0.0496 | 0.0410 | 0.0275 | 0.0095 |
| KS-eLDA | $(1/3, 1/3)$ | $E^{(0)}$ | 0.0014 | 0.0013 | 0.0012 | 0.0009 | 0.0003 | −0.0013 | −0.0079 |
| | | $E^{(1)}$ | 0.0149 | 0.0138 | 0.0115 | 0.0072 | −0.0001 | −0.0110 | −0.0209 |
| | | $E^{(2)}$ | 0.1217 | 0.1198 | 0.1154 | 0.1069 | 0.0917 | 0.0691 | 0.0389 |
| | | $\Omega^{(1)}$ | 0.0135 | 0.0125 | 0.0103 | 0.0063 | −0.0005 | −0.0096 | −0.0130 |
| | | $\Omega^{(2)}$ | 0.1203 | 0.1185 | 0.1142 | 0.1060 | 0.0914 | 0.0705 | 0.0469 |
| | | $\Upsilon_c^{(0)}$ | −0.0278 | −0.0270 | −0.0255 | −0.0227 | −0.0180 | −0.0105 | −0.0007 |
| | | $\Upsilon_c^{(1)}$ | −0.0034 | −0.0034 | −0.0037 | −0.0041 | −0.0050 | −0.0063 | −0.0076 |
| | | $\Upsilon_c^{(2)}$ | 0.0311 | 0.0304 | 0.0291 | 0.0268 | 0.0230 | 0.0168 | 0.0083 |
